# Supplementary material for: Broken sublattice symmetry states in Bernal stacked multilayer graphene
Source: arXiv:1610.07105 source file (2017-04-16)
Supplement: Supplementary file 1 [file supplemental.pdf]

# Supplemental Material:
# Broken sublattice symmetry states in Bernal stacked multilayer graphene

Chiho Yoon[1], Yunsu Jang[1], Jeil Jung[2], and Hongki Min[1]
[1] *Department of Physics and Astronomy, Seoul National University, Seoul 08826, Korea and*
[2] *Department of Physics, University of Seoul, Seoul 02504, Korea*

## I. FLAVOR ANTIFERRO STATES IN TETRALAYER GRAPHENE

From the Hartree energy cost considerations, the metastable states with the lowest total energy are expected to be flavor antiferro when there is no external electric field perpendicular to the graphene layers. Within the energetically more favorable flavor antiferro states, we classify different Hall phases [1, 2]: layer antiferromagnetic (LAF) phase with the spin dependent but valley independent sublattice potential, quantum spin Hall (QSH) phase with both the spin and valley dependent sublattice potential, and quantum anomalous Hall (QAH) phase with the valley dependent but spin independent sublattice potential, as schematically shown in Fig. 1.

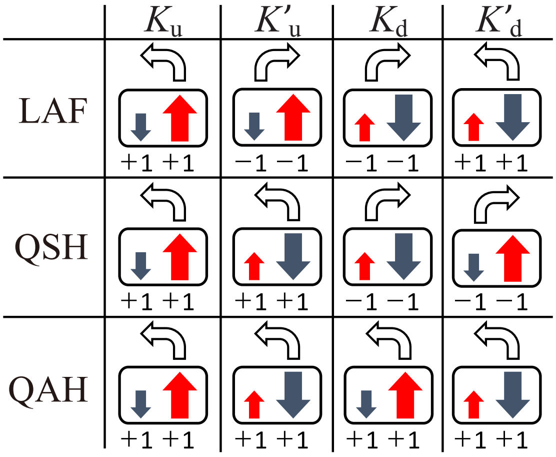


FIG. 1: Schematic picture of the ground-state configuration and corresponding spontaneous Hall effect at zero external electric field for three possible flavor antiferro states: LAF, QSH and QAH. Arrows in the square box and numbers below the box at each spin/valley flavor represent pseudospin polarizations and corresponding Chern numbers, respectively, whereas the arrows above the box indicate the corresponding net current directions expected in the Hall measurement.

The internal arrangement of the sublattice pseudospins has a direct impact on the Hall transport properties of the system. Whenever the charge polarization direction flips, the associated Chern number changes its sign due to the change in the sublattice potential in the doublet. We distinguish the spin Hall (SH), valley Hall (VH), charge Hall (CH), and spin resolved valley Hall (SV) contributions of the conductivities. From the Chern numbers $C_{v,s}$ ($v = K, K'$ and $s = \mathrm{u}, \mathrm{d}$) of the pseudospin doublets at each valley/spin flavor, the various quantum Hall conductivities can be evaluated as

$$\sigma_{\mathrm{SH}} = \frac{e^2}{h}\left(C_{K,\mathrm{u}} - C_{K,\mathrm{d}} + C_{K',\mathrm{u}} - C_{K',\mathrm{d}}\right), \tag{1a}$$

$$\sigma_{\mathrm{VH}} = \frac{e^2}{h}\left(C_{K,\mathrm{u}} + C_{K,\mathrm{d}} - C_{K',\mathrm{u}} - C_{K',\mathrm{d}}\right), \tag{1b}$$

$$\sigma_{\mathrm{CH}} = \frac{e^2}{h}\left(C_{K,\mathrm{u}} + C_{K,\mathrm{d}} + C_{K',\mathrm{u}} + C_{K',\mathrm{d}}\right), \tag{1c}$$

$$\sigma_{\mathrm{SV}} = \frac{e^2}{h}\left(C_{K,\mathrm{u}} - C_{K,\mathrm{d}} - C_{K',\mathrm{u}} + C_{K',\mathrm{d}}\right). \tag{1d}$$

Table I shows the resulting Hall conductivities for three distinct energy degenerate configurations (LAF, QSH, QAH) of the flavor antiferro phase.

TABLE I: Spontaneous quantum Hall conductivities in units of $e^2/h$ for the antiferro states in Bernal stacked tetralayer graphene under a perpendicular external electric field. Here, $E_{c1} = 0.025$ mV/Å and $E_{c2} = 0.879$ mV/Å.

| $E_{ext}$ | LAF | | | | QSH | | | | QAH | | | |
|---|---|---|---|---|---|---|---|---|---|---|---|---|
| | SH | VH | CH | SV | SH | VH | CH | SV | SH | VH | CH | SV |
| $E_{c2}$ | 0 | 0 | 0 | 0 | 0 | 0 | 0 | 0 | 0 | 0 | 0 | 0 |
| $E_{c1}$ | 0 | $-4$ | 0 | 4 | 4 | $-4$ | 0 | 0 | 0 | $-4$ | 4 | 0 |
| 0 | 0 | 0 | 0 | 8 | 8 | 0 | 0 | 0 | 0 | 0 | 8 | 0 |
| $-E_{c1}$ | 0 | 4 | 0 | 4 | 4 | 4 | 0 | 0 | 0 | 4 | 4 | 0 |
| $-E_{c2}$ | 0 | 0 | 0 | 0 | 0 | 0 | 0 | 0 | 0 | 0 | 0 | 0 |

## II. FLAVOR FERRI AND FERRO STATES IN TETRALAYER GRAPHENE

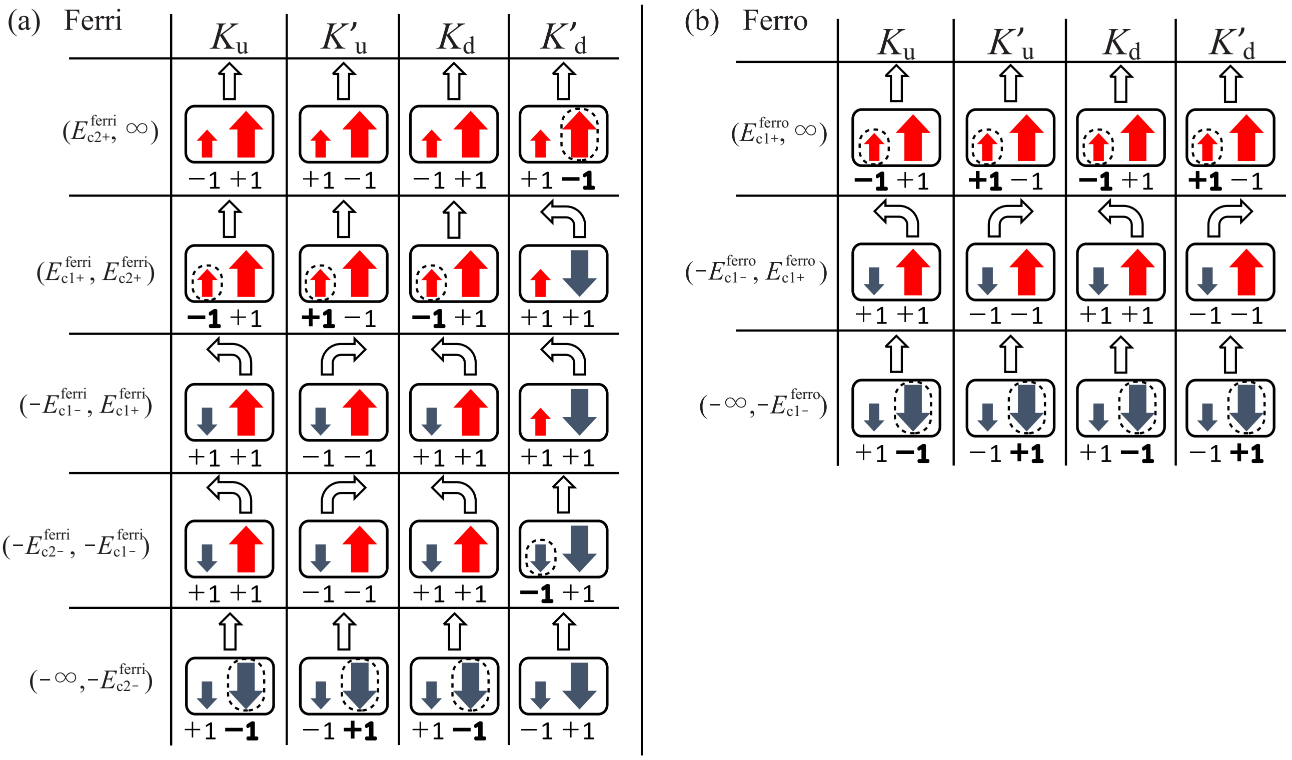


FIG. 2: The evolution of ABAB tetralayer graphene under a perpendicular external electric field for (a) a flavor ferri state with the minority pseudospin configuration (↑, ⇓) on $K'_d$ and (b) a flavor ferro state with (↓, ⇑) for all four flavors. Arrows in the square box and numbers below the box at each spin/valley flavor represent pseudospin polarizations and corresponding Chern numbers, respectively, whereas the arrows above the box indicate the corresponding net current directions expected in the Hall measurement. The change in the charge polarization by applying a perpendicular electric field is denoted by the dashed circle.

As demonstrated in the main text, the ground-state configurations of tetralayer graphene and their field dependence can be clearly explained by the effective "Hund's rule". The evolution of a flavor ferri state with the minority pseudospin configuration on $K'_d$ and that of a flavor ferro state under a perpendicular external electric field are depicted in Fig. 2. The corresponding Chern numbers for each state are represented in Tab. II. Note that in zero external electric field, there are eight ferri states (from the two possible choice of minority configuration between (↑,⇓) and (↓,⇑) on four possible spin/valley flavors) and two ferro states (from the two possible choice of majority configuration).

As shown in Table II, in the case of ferri states, all the types of Hall coefficients are non-zero for $-E^{\rm ferri}_{c2-} < E < E^{\rm ferri}_{c2+}$. This is the reason why the ferri state is also called "All" state [1–3]. Also note that only the valley Hall coefficients

TABLE II: Spontaneous quantum Hall conductivities in units of $e^2/h$ under a perpendicular external electric field in ABAB tetralayer for the ferri and ferro states in Fig. 2. Here, $E_{c1+}^{\text{ferri}} = 0.019$, $E_{c2+}^{\text{ferri}} = 0.943$, $E_{c1-}^{\text{ferri}} = 0.031$, and $E_{c2-}^{\text{ferri}} = 0.815$ meV/Å for the ferri state, whereas $E_{c1+}^{\text{ferro}} = 0.013$ and $E_{c1-}^{\text{ferro}} = 0.753$ meV/Å for the ferro state.

| $E$ | Ferri | | | |
|---|---|---|---|---|
| | SH | VH | CH | SV |
| $E_{c2+}^{\text{ferri}}$ | 0 | 0 | 0 | 0 |
| $E_{c1+}^{\text{ferri}}$ | $-2$ | $-2$ | 2 | 2 |
| 0 | $-4$ | 4 | 4 | 4 |
| $-E_{c1-}^{\text{ferri}}$ | $-2$ | 6 | 2 | 2 |
| $-E_{c2-}^{\text{ferri}}$ | 0 | 0 | 0 | 0 |

| $E$ | Ferro | | | |
|---|---|---|---|---|
| | SH | VH | CH | SV |
| $E_{c1+}^{\text{ferro}}$ | 0 | 0 | 0 | 0 |
| 0 | 0 | 8 | 0 | 0 |
| $-E_{c1-}^{\text{ferro}}$ | 0 | 0 | 0 | 0 |

change their signs in the opposite field direction. In the case of ferro states, only the valley Hall coefficients are non-zero for $-E_{c1-}^{\text{ferro}} < E < E_{c1+}^{\text{ferro}}$.

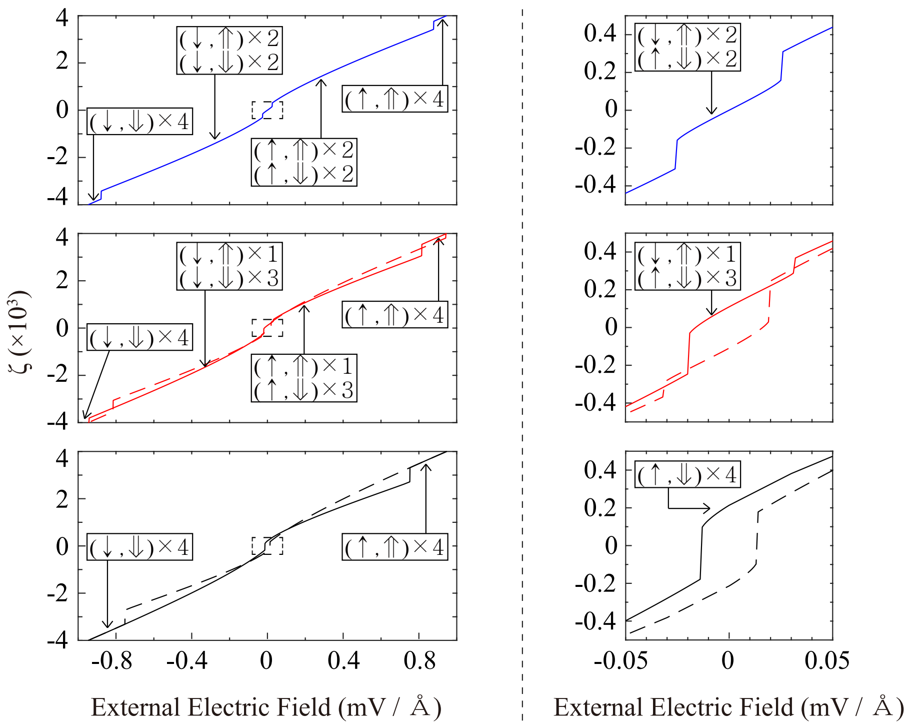


FIG. 3: (Left) External field dependence of the total charge polarization $\zeta$ defined in Eq. (2) for flavor antiferro (top), ferri (middle) and ferro (bottom) states. The solid and dashed lines indicate evolutions of states from two different initial states with reversed polarization direction for each pseudospin. For each solid line, the pseudospin configurations are depicted. (Right) Zoomed view of the dashed rectangular area in the left panel.

Figure 3 shows the external field dependence of the total charge polarization for flavor antiferro, ferri and ferro states tracing a single metastable configuration. Here, we define the total charge polarization $\zeta$ in tetralayers taking into account the layer separations as

$$\zeta = \frac{\frac{3}{2}n_4 + \frac{1}{2}n_3 - \frac{1}{2}n_2 - \frac{3}{2}n_1}{n_4 + n_3 + n_2 + n_1}, \tag{2}$$

where $n_i$ is the electron density at $i$-th layer. Note that in the case of ferri and ferro states, the evolution of states depends on the initial condition and the sweep direction of the field, exhibiting hysteretic behavior associated with the broken sublattice symmetry at zero field, which is analogous to the bilayer graphene system [4].

TABLE III: Charge polarizations and corresponding Chern numbers in the presence of a perpendicular electric field in Bernal stacked 6-layer graphene for the LAF state. The pseudospins are written in increasing effective mass order from the left to the right. Here, $E_{c1}^{(6)} = 0.017$, $E_{c2}^{(6)} = 0.251$, and $E_{c3}^{(6)} = 0.281$ meV/Å. Red arrows indicate flipped pseudospin polarizations with field.

| $E$ | Flavor I ($K_u$, $K'_u$) | | | Flavor II ($K_d$, $K'_d$) | | | Chern Number | | | |
|---|---|---|---|---|---|---|---|---|---|---|
| | | | | | | | $K_u$ | $K_d$ | $K'_u$ | $K'_d$ |
| $E_{c3}^{(6)}$ | ↑ | ↑ | ↑ | ↑ | ↑ | ↑ | 1 | 1 | −1 | −1 |
| $E_{c2}^{(6)}$ | ↑ | ↑ | ↑ | ↑ | ↑ | ↓ | 1 | −1 | −1 | 1 |
| $E_{c1}^{(6)}$ | ↑ | ↓ | ↑ | ↑ | ↑ | ↓ | 3 | −1 | −3 | 1 |
| 0 | ↑ | ↓ | ↑ | ↓ | ↑ | ↓ | 3 | −3 | −3 | 3 |
| $-E_{c1}^{(6)}$ | ↓ | ↓ | ↑ | ↓ | ↑ | ↓ | 1 | −3 | −1 | 3 |
| $-E_{c2}^{(6)}$ | ↓ | ↓ | ↑ | ↓ | ↓ | ↓ | 1 | −1 | −1 | 1 |
| $-E_{c3}^{(6)}$ | ↓ | ↓ | ↓ | ↓ | ↓ | ↓ | −1 | −1 | 1 | 1 |

TABLE IV: Spontaneous quantum Hall conductivities in units of $e^2/h$ for the antiferro states in Bernal stacked 6-layer graphene under a perpendicular external electric field.

| $E_{ext}$ | LAF | | | | QSH | | | | QAH | | | |
|---|---|---|---|---|---|---|---|---|---|---|---|---|
| | SH | VH | CH | SV | SH | VH | CH | SV | SH | VH | CH | SV |
| $E_{c3}^{(6)}$ | 0 | 4 | 0 | 0 | 0 | 4 | 0 | 0 | 0 | 4 | 0 | 0 |
| $E_{c2}^{(6)}$ | 0 | 0 | 0 | 4 | 4 | 0 | 0 | 0 | 0 | 0 | 4 | 0 |
| $E_{c1}^{(6)}$ | 0 | 4 | 0 | 8 | 8 | 4 | 0 | 0 | 0 | 4 | 8 | 0 |
| 0 | 0 | 0 | 0 | 12 | 12 | 0 | 0 | 0 | 0 | 0 | 12 | 0 |
| $-E_{c1}^{(6)}$ | 0 | −4 | 0 | 8 | 8 | −4 | 0 | 0 | 0 | −4 | 8 | 0 |
| $-E_{c2}^{(6)}$ | 0 | 0 | 0 | 4 | 4 | 0 | 0 | 0 | 0 | 0 | 4 | 0 |
| $-E_{c3}^{(6)}$ | 0 | −4 | 0 | 0 | 0 | −4 | 0 | 0 | 0 | −4 | 0 | 0 |

## III. GROUND-STATE CONFIGURATIONS FOR 6-LAYER GRAPHENE

Similarly as tetralayer graphene, the low-energy band structure of Bernal stacked 6-layer graphene (ABABAB) at low energies is described by three bilayer-like pseudospin doublets with different masses. Because of the sublattice symmetry breaking, charge polarizations of the three pseudospins have alternating directions, (↓,↑,↓) or (↑,↓,↑) where arrows in the parenthesis represent the charge polarization of pseudospins with increasing effective mass order. The corresponding Chern numbers are (+1,+1,+1) or (−1,−1,−1) because of the same sign of sublattice potential generated by the sublattice symmetry breaking. Similarly, we can understand the ground-state configurations of 8-layer graphene (ABABABAB) as (↓,↑,↓,↑) or (↑,↓,↑,↓) with the Chern numbers (+1,+1,+1,+1) or (−1,−1,−1,−1) at zero field.

Table III shows the external field dependence of the ground-state configurations in the LAF state for 6-layer graphene. In Tab. IV, the corresponding Hall conductivities are calculated for the three possible antiferro states, respectively. When the external electric field $E_{ext}$ is zero, pseudospins with increasing effective mass have alternating charge polarization directions for 6-layer graphene, which is consistent with the tetralayer case. As $E_{ext}$ increases, each pseudospin flips from the one with lighter effective mass following the Hund's rule. As the number of layers increases, however, there are deviations from this rule in the intermediate field region resulting from the greater complexity of the intermediate states and the interaction between the bands near the Fermi energy.

## IV. EFFECT OF THE REMOTE HOPPING TERMS

In even-layer graphenes, the energy gap is the dominant energy scale, thus when the gap is large enough, the effect of other energy scales associated with remote hopping terms could be negligible and the basic picture presented in this paper remains valid at least qualitatively. However, when the remote hopping terms are not negligible compared to the energy gap, the ground state is no longer described by the sublattice symmetry breaking and the effective Hund's rule, and the detailed ground state configurations will be determined by combined effects of the remote hopping terms and screening. Figure 4 shows the phase diagram between the gap dominant and remote-hopping dominant regions as a function of the interaction strength $\alpha$ and the next-nearest interlayer coupling between non-dimer sites $\gamma_2$ in

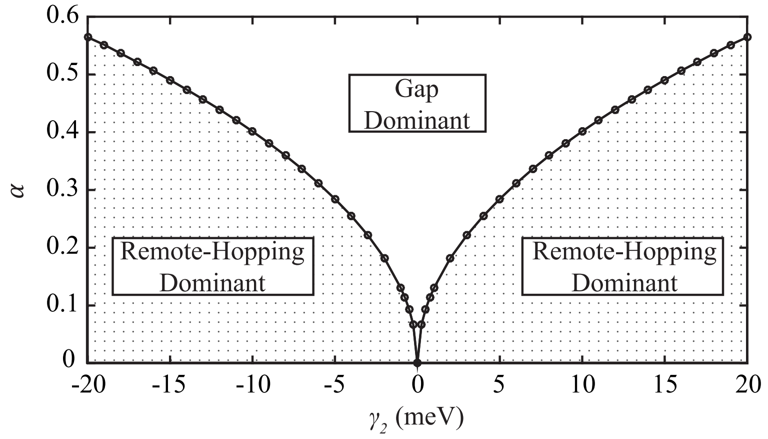


FIG. 4: The phase diagram for the ground state configuration of tetralayer graphene on $\alpha$ and $\gamma_2$ plane. Here, the gap (remote-hopping) dominant region denotes a region where the ground state is (not) described by the sublattice symmetry breaking and the effective Hund's rule.

tetralayer graphene, ignoring the other remote hopping terms for simplicity. In the gap (remote-hopping) dominant region, the ground state is (not) described by the sublattice symmetry breaking and the effective Hund's rule. As expected, broken sublattice symmetry occurs at large $\alpha$ and small size of $\gamma_2$. If we adopt the proposal that the remote hopping terms in multilayer graphene are different from those in graphite and are suppressed by interaction induced strains [5], the use of the minimal model for the band Hamiltonian would be justified. Considering that $\alpha \sim 1$ for conventional $SiO_2$ substrates and $\alpha \sim 2.6$ for suspended samples for the dielectric environment, we expect a fair chance that the gap dominant region prevails over the remote hopping dominant region. The fact that a rather weaker $\alpha \sim 0.1$ in our modeling gives a reasonable description of the experiments indicates that the quantitative value of the band gap contains a combined effect of interaction screening and band Hamiltonian effects that should be accounted for in a more complete theory.

[1] F. Zhang, J. Jung, G. A. Fiete, Q. Niu, and A. H. MacDonald, Phys. Rev. Lett. **106**, 156801 (2011).
[2] J. Jung, F. Zhang, and A. H. MacDonald, Phys. Rev. B **83**, 115408 (2011).
[3] F. Zhang, Synth. Met. **210**, 9 (2015).
[4] H. Min, G. Borghi, M. Polini, and A. H. MacDonald, Phys. Rev. B **77**, 041407(R) (2008).
[5] Y. Nam, D.-K. Ki, M. Koshino, E. McCann, and A. F. Morpurgo, 2D Mater. **3**, 045014 (2016).
